# Supplementary material for: Multi-source adversarial transfer learning based on similar source domains with local features
Source: arXiv:2305.19067 source file (2023-06-29)
Supplement: Supplementary file 1 [file appendix.tex]

\newpage
\section{附录}
%表\ref{Benign_IoU_score_result},表\ref{Benign_Dice_score_result},表\ref{Benign_F2_score_result},表\ref{Benign_F05_score_result}分别给出了BUSI Benign作为目标域的$IoU$,$Dice \ score$,$F_{2}$$F_{0.5}$结果；
%表\ref{Malignant_IoU_score_result} ,表\ref{Malignant_Dice_score_result},表\ref{Malignant_F2_score_result},表\ref{Malignant_F05_score_result}分别给出了BUSI Malignant作为目标域的$IoU$,$Dice \ score$,$F_{2}$,$F_{0.5}$结果。
\input{tables/Benign_score_result.tex}
\input{tables/Malignant_score_result.tex}
